# Supplementary material for: Coupled imbibition and evaporation of droplets deposited on a nanoporous layer
Source: arXiv:2510.19932 ancillary file (2026-01-05)
Supplement: Supplementary file 1 [file SuppMat.pdf]

# Coupled imbibition and evaporation of droplets deposited on a nanoporous layer

—

## Supporting Information

Joachim Trosseille, Hugo Bellezza, and Olivier Vincent*

*Universite Claude Bernard Lyon 1, CNRS, Institut Lumière Matière, UMR5306, F-69100, Villeurbanne, France*

E-mail: olivier.vincent@cnrs.fr

# Contents

**S1 Sample characterization** 1
- S1.1 Water sorption isotherms . . . . . 1
- S1.2 Pore size distribution . . . . . . . 2
- S1.3 Equilibrium and condensation RH 3
- S1.4 Capillary pressure . . . . . . . . . 3
- S1.5 Porosity and thickness . . . . . . 3

**S2 Image analysis** 4
- S2.1 Droplet and halo contours . . . . 4
- S2.2 Droplet shape measurement . . . 5

**S3 Numerical estimates** 8
- S3.1 Water properties . . . . . . . . . 8
- S3.2 Lucas-Washburn coefficient . . . . 8
- S3.3 Droplet: initial transient . . . . . 8

**S4 Misc. discussion** 9
- S4.1 Fitting of halo dynamics . . . . . 9
- S4.2 Dynamic vs. equilibrium humidity 9

**References** 10

# S1 Sample characterization

We measured water sorption isotherms by white light interferometry (WLI), from which we extracted the thickness and porosity of the material, and estimated the capillary pressure and pore size distribution. We also used an alternative method to measure porosity, based on the evaluation of the final concentration of an aqueous solution infiltrated in the pore space.

## S1.1 Water sorption isotherms

We measured water sorption isotherms on our sample using white light interferometry (WLI). The WLI setup and analysis procedure are described elsewhere.[1] Briefly, the method is based on the analysis of reflected spectra with white light illumination; due to optical interference between optical rays reflected on top and at the bottom of the porous layer, the spectra are modulated with a periodicity that depends on the optical path length,

$$\mathcal{L} = 2nH \tag{S1}$$

where $n$ is the refractive index of the layer, and $H$ its thickness. When water evaporates or condenses due to relative humidity (RH) decrease or increase, $n$ changes, resulting in variations in $\mathcal{L}$ that are linear with the filling fraction of the pores, $f$, to very good approximation.[2,3]

Figure S1a presents an isotherm obtained

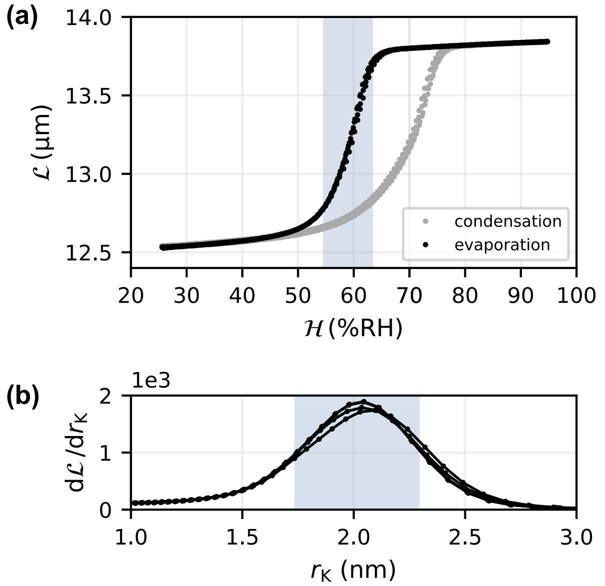


Figure S1: (a) Water isotherm obtained by white light interferometry (WLI), with 4 successive cycles overlapped. Condensation branches correspond to increasing RH, and evaporation branches to decreasing RH. (b) Distribution of Kelvin radii extracted from the evaporation branch of the isotherm. The shaded, blue areas in both panels indicate the estimated range of equilibrium RH (panel a) and Kelvin radius (panel b).

with the WLI method, where we monitored changes in optical path length while the sample underwent 4 successive cycles of relative humidity between 25 %RH ($\mathcal{H} = p/p_{\mathrm{sat}} = 0.25$) and 95 %RH ($\mathcal{H} = 0.95$), with a rate of change of 0.5 %RH / min ($\mathrm{d}\mathcal{H}/\mathrm{d}t = 8.33 \times 10^{-5}\,\mathrm{s}^{-1}$). We extracted the extrema values of optical path length, $\mathcal{L}_{\mathrm{empty}} = 12.47\,\mu\mathrm{m}$ and $\mathcal{L}_{\mathrm{full}} = 13.85\,\mu\mathrm{m}$ by extrapolation of the WLI data as in Figure S1a to 0%RH and 100%RH, respectively. Using the assumption of linear variations of optical path length with the filling fraction of the porous layer,[2,3] we use the formula

$$f = \frac{\mathcal{L} - \mathcal{L}_{\mathrm{empty}}}{\mathcal{L}_{\mathrm{full}} - \mathcal{L}_{\mathrm{empty}}} \qquad \text{(S2)}$$

to estimate the filling fraction of the porous layer and to generate the filling fraction isotherm shown in the Main Text.

## S1.2 Pore size distribution

We also estimated the pore size distribution in our sample using the Kelvin-Laplace equation that relates the equilibrium radius of curvature $r_{\mathrm{K}}$ (*Kelvin radius*), of liquid-vapor menisci to the relative humidity:

$$r_{\mathrm{K}} = -\frac{2\gamma v_{\mathrm{m}}}{\bar{R}T\ln(\mathcal{H})} \qquad \text{(S3)}$$

with $v_{\mathrm{m}}$ the molar volume of the liquid ($\mathrm{m}^3$/mol), $\gamma$ the surface tension of the liquid/vapor interface (N/m), $\bar{R}$ the ideal gas constant ($\mathrm{J\,mol^{-1}\,K^{-1}}$) and $T$ temperature (K). We apply this equation to the evaporation branch of the isotherm, where it is commonly assumed that pores contain spherical-cap shaped menisci and empty at equilibrium.[4] Using Equation S3 we can transform the $\mathcal{L}(\mathcal{H})$ isotherm into a $\mathcal{L}(r_{\mathrm{K}})$ curve; we then differentiate $\mathcal{L}(r_{\mathrm{K}})$ to obtain a representation of the distribution of equilibrium Kelvin radii in our sample. Figure S1b presents the result of this analysis, with a typical range

$$r_{\mathrm{K}} = (2.01 \pm 0.28)\,\mathrm{nm} \qquad \text{(S4)}$$

obtained from the full width at half maximum of the obtained distribution (shaded, blue area).

Note that $r_{\mathrm{K}}$ is not directly the geometrical pore size, which can be estimated using Laplace's law

$$r_{\mathrm{p}} = r_{\mathrm{K}} \cos\theta_{\mathrm{e}} \qquad \text{(S5)}$$

where $\theta_{\mathrm{e}}$ is the equilibrium contact angle.[1] In order to estimate $r_{\mathrm{p}}$, we use for $\theta_{\mathrm{e}}$ the initial contact angle $\theta \simeq 27°$ observed for water droplets in our experiments (see Main Text), which we assume to be close to the equilibrium contact angle of water on the pore walls. Using Equation S5, we have

$$r_{\mathrm{p}} \simeq (1.79 \pm 0.25)\,\mathrm{nm} \qquad \text{(S6)}$$

which should be taken as an approximate pore radius, given the potential effects of confinement on macroscopic laws such as Laplace and Kelvin, and effects of the pore size distribution.

## S1.3 Equilibrium and condensation RH

From the extracted range of $r_\mathrm{K}$, we calculated a range of equilibrium RH through Equation S3,

$$\mathcal{H}_\mathrm{eq} = 0.590 \pm 0.043 \qquad \text{(S7)}$$

(relative humidity in the range 54.7–63.3 %RH), see shaded blue area in Figure S1a.

We also estimated a typical range of condensation RH by taking the range of optical path length $\mathcal{L}$ corresponding to the range of equilibrium RH on the *evaporation* branch of the isotherm, and calculated the range of RH on the *condensation* branch of the isotherm corresponding to the same variations in $\mathcal{L}$. We obtained

$$\mathcal{H}_\mathrm{cond} = 0.684 \pm 0.059 \qquad \text{(S8)}$$

(relative humidity in the range 62.5–74.3 %RH).

## S1.4 Capillary pressure

We also estimated from the extracted distribution of $r_\mathrm{K}$ the equilibrium capillary pressure in the pores, using Laplace's law

$$\Delta P_\mathrm{c} = \frac{2\gamma}{r_\mathrm{K}} \qquad \text{(S9)}$$

resulting in $\Delta P_\mathrm{c} = (-72.7 \pm 9.9)\,\mathrm{MPa}$.

## S1.5 Porosity and thickness

We estimated the porosity of the porous layer, $\phi$, using two methods: effective medium optics based on WLI data, and salt concentration. The WLI method also allowed us to measure the thickness of the porous layer, $H$.

**WLI effective medium optics** With this method, we evaluate porosity, $\phi$, and thickness $H$ of the porous layer based on the difference in measured optical path length, $\mathcal{L}$ between a dry sample ($\mathcal{L}_\mathrm{empty}$), and a fully wet sample ($\mathcal{L}_\mathrm{full}$).

We use the Bruggeman effective medium approach to describe the optical response of the porous medium as a function of its porosity, $\phi$, and filling fraction, $f$ ($f = 0$ when the pores are empty, and $f = 1$ when they are full of water). Within this framework, the average index of refraction, $n$, of the porous medium follows[5,6]

$$(1-\phi)\frac{\epsilon_\mathrm{s}-\epsilon}{\epsilon_\mathrm{s}+2\epsilon} + \phi f \frac{\epsilon_\mathrm{w}-\epsilon}{\epsilon_\mathrm{w}+2\epsilon} + \phi(1-f)\frac{1-\epsilon}{1+2\epsilon} = 0 \qquad \text{(S10)}$$

where $\epsilon = n^2$, and where $\epsilon_\mathrm{w} = n_\mathrm{w}^2$ and $\epsilon_\mathrm{s} = n_\mathrm{s}^2$ correspond to the liquid (water), and the solid (silica), respectively.

Equation S10 reduces to

$$\frac{\epsilon_\mathrm{s}-\epsilon_\mathrm{empty}}{\epsilon_\mathrm{s}+2\epsilon_\mathrm{empty}} = \left(\frac{\phi}{\phi-1}\right)\frac{1-\epsilon_\mathrm{empty}}{1+2\epsilon_\mathrm{empty}} \qquad \text{(S11)}$$

when the pores are empty ($f = 0$), and to

$$\frac{\epsilon_\mathrm{s}-\epsilon_\mathrm{full}}{\epsilon_\mathrm{s}+2\epsilon_\mathrm{full}} = \left(\frac{\phi}{\phi-1}\right)\frac{\epsilon_\mathrm{w}-\epsilon_\mathrm{full}}{\epsilon_\mathrm{w}+2\epsilon_\mathrm{full}} \qquad \text{(S12)}$$

when the pores are full ($f = 1$). In Equations S11 and S12, we can replace $\epsilon_\mathrm{empty}$ and $\epsilon_\mathrm{full}$ by $\sqrt{\mathcal{L}_\mathrm{empty}/(2H)}$ and $\sqrt{\mathcal{L}_\mathrm{full}/(2H)}$ respectively, using Equation S1. Using the measured values of $\mathcal{L}_\mathrm{empty}$ and $\mathcal{L}_\mathrm{full}$ and Equations S11-S12, we can thus extract independently the porosity and the porous layer thickness if we assume a known value for the index of refraction of the solid. Using $n_\mathrm{s} = \epsilon_\mathrm{s}^2 = 1.45 \pm 0.05$ for silica[7,8] (we expect the pore walls to be made of silica, see *Methods* in main text), we obtain $\phi = 0.404 \pm 0.006$ and $H = (4.95 \pm 0.10)\,\mu\mathrm{m}$. These values are in excellent agreement with expectations for oxidized porous silicon samples[9–11] and with the concentration method discussed below; they also indicate that the values of porosity and layer thickness that are extracted from the measurements are only weakly dependent on the actual choice of index of refraction of silica.

**Concentration method** We prepared an aqueous solution of sodium chloride (NaCl) of concentration, $C_\mathrm{init}$ = 0.515 mol/L. We deposited a droplet volume, $V_\mathrm{init} = 2\,\mu\mathrm{L}$ of that solution on the sample close to its center, while maintaining the relative humidity high enough to have the pores always full due to capillary condensation. Due to diffusion, the salt progressively invaded the pore space, while the

droplet shrank due to evaporation until disappearance. We let the system equilibrate overnight, after which we assumed that the salt concentration was uniform in the whole porous layer (a typical diffusion time is $L^2/D_s \simeq 3.5$ hours with $L = 5\,\mathrm{mm}$ and $D_s \simeq 2 \times 10^{-9}\,\mathrm{m^2/s}$). We then measured the water activity of the pore solution, $a_w$, using water sorption isotherms; this in-situ calibration method is described elsewhere.[1] By repeating sorption isotherms, we could check that the extracted value of $a_w \simeq 0.766 \pm 0.014$ was stable across cycles, showing that the system was indeed equilibrated.

We then used known correlations for water activity as a function of molality[12] and for density as a function of salt concentration[13] to calculate the concentration (molarity), $C_{\mathrm{pores}}$mol/L, of the pore solution. We obtained $C_{\mathrm{pores}} = (5.20 \pm 0.23)\,\mathrm{mol/L}$. From this value, we could calculate the pore volume using the conservation of amount of salt, $C \times V = \mathrm{const}$:

$$V_{\mathrm{pores}} = V_{\mathrm{init}} \frac{C_{\mathrm{init}}}{C_{\mathrm{pores}}} \tag{S13}$$

leading to $V_{\mathrm{pores}} = (0.198 \pm 0.009)\,\mathrm{\mu L}$.

We finally obtained the porosity,

$$\phi = \frac{V_{\mathrm{pores}}}{V_{\mathrm{tot}}} \tag{S14}$$

with $V_{\mathrm{tot}}$ the total volume of the porous layer, which we estimated from the exposed area, $A = 102\,\mathrm{mm^2}$ (obtained from image analysis) and layer thickness, $H = (4.95 \pm 0.10)\,\mathrm{\mu m}$ obtained with the WLI method (see above), leading to $V_{\mathrm{tot}} = A \times H = (0.51 \pm 0.01)\,\mathrm{\mu L}$. Finally from Equation S14 we obtain $\phi = 0.39 \pm 0.02$

**Conclusion** From the different methods above, a value of porosity

$$\phi = 0.39 \pm 0.02 \tag{S15}$$

encompasses the range of obtained values from the concentration method and from the effective medium optics method. We have also measured

$$H = (4.95 \pm 0.10)\,\mathrm{\mu m} \tag{S16}$$

for the porous layer thickness.

# S2 Image analysis

## S2.1 Droplet and halo contours

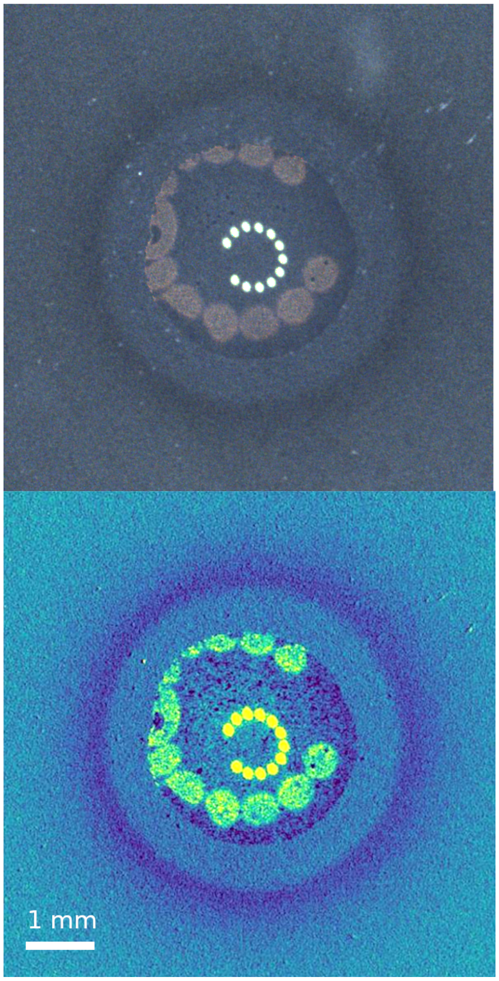


Figure S2: Preprocessing of images for contour detection. Top: raw image with slightly increased brightness and contrast. Bottom: background subtracted image with viridis pseudocolor scale.

From images such as in Figure 1b in the main text, we determined the droplet base radius, $R_{\mathrm{drop}}$ and the position of the imbibition halo using a semi-manual method. The latter consists in a automated treatment of images including a manual detection step of the position of the halo. Indeed, due to a poor contrast of the original images (see figure S2), the halo just induces a slight change of the gray level of the image, making it hard to detect using traditional threshold based segmentation algorithms. Unless using a fastidious specific parameterization of the algorithm for each experiment, we were not able to catch the position of the halo with a

fully automatic process. Our method was however verified to be consistent with classical segmentation algorithm on selected datasets.

## S2.2 Droplet shape measurement

We calculate the contact angle, $\theta$, and volume, $V$, of the droplet from top-view images, taking advantage of the fact that optical reflections on top of the droplet change as a function of its shape, which we assume to be a spherical cap. In particular, we use the reflection of the LED illumination ring to measure the temporal evolution of $\theta$ and $V$.

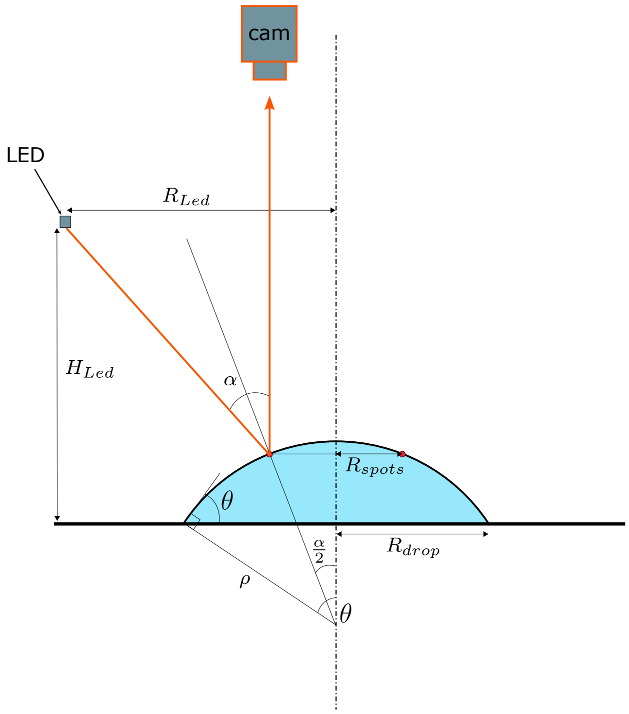


Figure S3: Schematic of a side view of the drop. The distances and angles used for the calculation of the contact angle of the drop, $\theta$, are indicated on the drawing. The positions of the camera and of the LED ring are not to scale.

Figure S3 shows a side view of the drop and the distances and angles used for the calculation of the contact angle, $\theta$, and subsequently the volume of the drop. The calculation is based on the fact that the distance $R_{\text{spots}}$, *i.e.* the position of the LED ring reflections as compared to the center of symmetry of the drop, depends on the contact angle of the drop. The following development assumes that the LED ring and the camera are far enough from the drop so that the incident and reflective light beam have always the same direction independently of the position of the spot.

The contact angle of the drop with the substrate is calculated from

$$\theta = \arcsin\left(\frac{R_{\text{drop}} \times \sin(\beta)}{R_{\text{spots}}}\right) \quad \text{(S17)}$$

with

$$\beta = \frac{1}{2} \times \arctan\left(\frac{R_{\text{LED}}}{H_{\text{LED}}}\right) \quad \text{(S18)}$$

The volume of the drop is then

$$V_{\text{drop}} = \pi R_{\text{drop}}^3 \times \frac{2 - 3\cos(\theta) + \cos^3(\theta)}{3\sin^3(\theta)} \quad \text{(S19)}$$

$R_{\text{drop}}$ is determined by calculating the coordinates of the intersection points between the measurement line and the ellipse. $R_{\text{spots}}$ is obtained from the profile of the measurement lines (see Figure S4) which exhibits two peaks corresponding to the center of two opposite dots as compared to the center of the drop (see Figure S5) The volume of the drop is calculated for each measurement line in Figure S4, then averaged to get the total volume.

Figure S6 shows the evolution of the drop during evaporation. The droplet volume is calculated from the evolution of the distance between reflection dots at the surface of the drop. There is a first regime with constant base radius, from $t = 2$ s to $t = 293$ s, where the contact line is pinned. The base radius of the drop stays constant while the contact angle decreases. The contact line then detaches and the drop enters in a regime of constant contact angle evaporation, while the radius decreases. The measurement of volume is only made in the constant radius regime.

Typical evolution of the drop contact angle $\theta$ as calculated from equation S17 and subsequent volume of the drop as calculated from equation S19 are shown in figure S7.

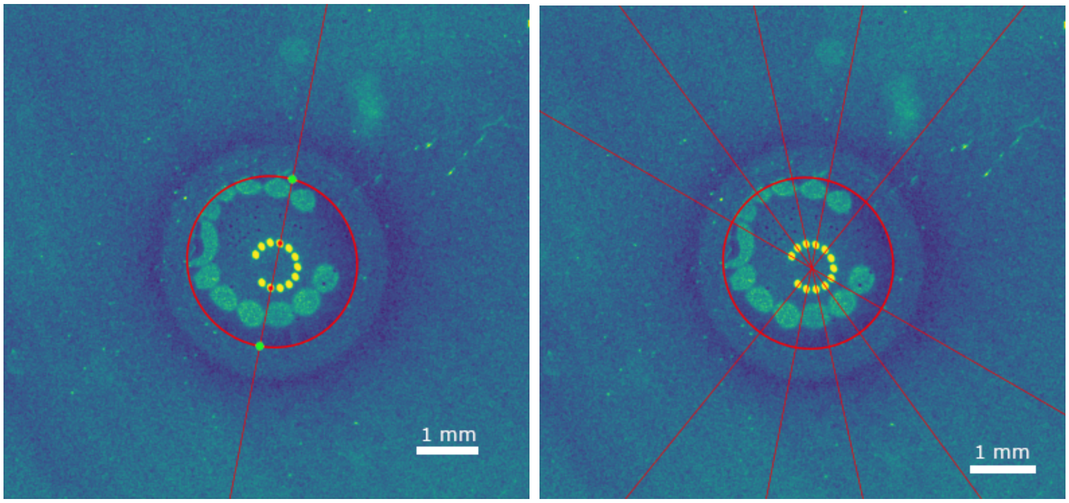


Figure S4: Typical image for analysis ($t$ = 20 s). Left: the red circle represents the edge of the drop, that is the contact line with the solid. The straight red line is the measurement line where the detection of the spacing between two opposite reflection dots is performed, as well as the estimation of the width of the drop. The red dots correspond to the intersections between the straight line and the contact line of the drop; their spacing is $D_{\text{drop}}$. Red dots are the positions of the reflection dots on the measurement line; Their spacing is $D_{\text{spots}}$. Right: position of the five measurement lines.

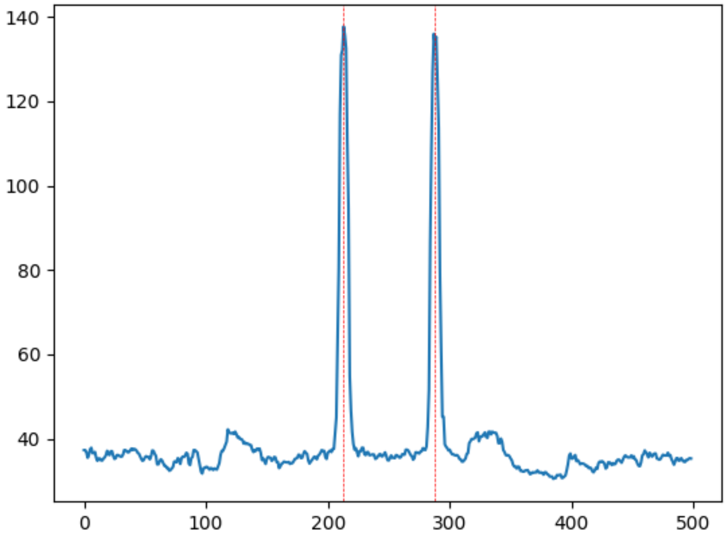


Figure S5: Exemple of a mean profile along a measurement line. The two peaks correspond to the center of the reflection of the LED illumination on the drop. Their spacing is $D_{\text{spots}}$.

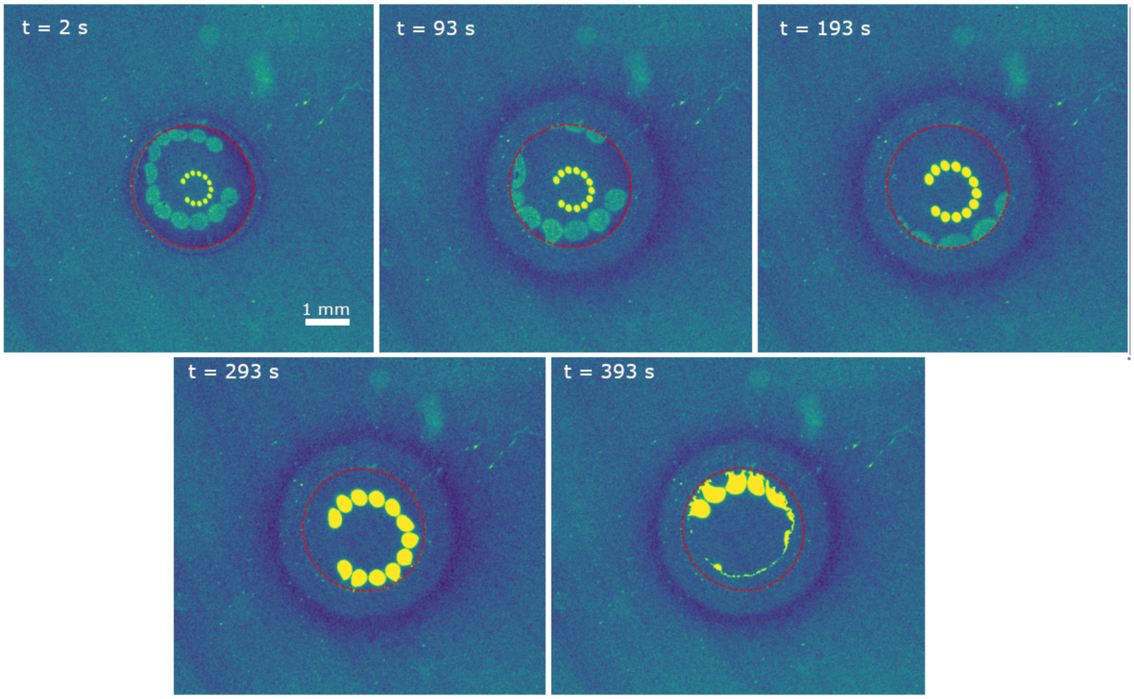


Figure S6: Evolution of the drop during evaporation. Red interrupted line: initial position of the contact line. Yellow dots: reflections of the LED illumination at the surface of the drop, which we use to calculate the droplet volume.

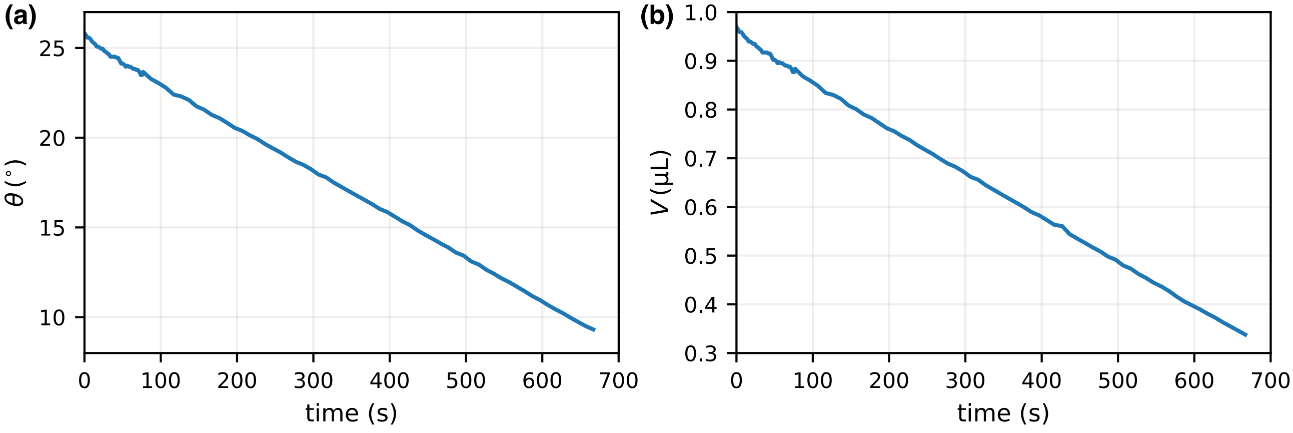


Figure S7: Droplet geometry inferred from LED reflections. (a) Contact angle $\theta$ as a function of time, and (b) corresponding droplet volume during evaporation. The measurement stops when the contact line starts receding (depinning). The data shown here is for an experiment done at 70 %RH.

# S3 Numerical estimates

## S3.1 Water properties

We have used correlations from the literature to calculate the properties of water and estimate their associated uncertainties based on the typical variations of temperature in our experiments, $T = (24.3 \pm 0.4)\,°\mathrm{C}$. We have used equations recommended by the International Association for the Properties of Water and Steam (IAPWS) for liquid water density at atmospheric pressure,[14] saturation vapor pressure[15] and surface tension.[16] From the density, $\rho$, we also calculate the molar volume of water, $v_\mathrm{m} = M/\rho$, where $M = 0.018015268$ kg/mol is the molar mass of water. From the molar volume and saturation vapor pressure $p_\mathrm{sat}$, we also obtain the dimensionless parameter $\epsilon = v_\mathrm{m} p_\mathrm{sat}/(\bar{R}T)$ (with $\bar{R} = 8.314\,462\,\mathrm{J\,mol^{-1}\,K^{-1}}$ the ideal gas constant and $T$ expressed in K), which corresponds to the density ratio between water vapor and liquid water at saturation. Finally, we also use a correlation provided by Massman for the diffusivity of water vapor in air as a function of temperature.[17] All these values can also be obtained using the *aquasol* Python package,[18] which provides direct programming access to the formula above. The corresponding values are listed in Table 1

Table 1: Numerical values for water properties.

| | Symbol | Value | Unit |
|---|---|---|---|
| Density | $\rho$ | $997.224 \pm 0.010$ | $\mathrm{kg/m^3}$ |
| Molar volume | $v_\mathrm{m}$ | $(1.8066 \pm 0.0002) \times 10^{-5}$ | $\mathrm{m^3/mol}$ |
| Saturation vapor pressure | $p_\mathrm{sat}$ | $3041 \pm 73$ | Pa |
| Density ratio | $\epsilon$ | $(2.22 \pm 0.05) \times 10^{-5}$ | – |
| Diffusivity in air | $D$ | $(2.54 \pm 0.01) \times 10^{-5}$ | $\mathrm{m^2/s}$ |
| Surface tension | $\gamma$ | $(72.08 \pm 0.06) \times 10^{-3}$ | N/m |

## S3.2 Lucas-Washburn coefficient

In order to estimate the Lucas-Washburn (LW) transport parameter, $w$, of water in our porous silicon material, we use the formula

$$w = \frac{2\kappa|\Delta P_\mathrm{c}|}{\phi} \tag{S20}$$

(see main text). For the porosity, we use the value, $\phi = 0.39 \pm 0.02$ estimated above. For the capillary pressure, we use $\Delta P_\mathrm{c} = (-72.7 \pm 9.9)$ MPa as obtained from water sorption isotherms (see above). While we do not have a direct measurement of the permeability, $\kappa$, on our material, its fabrication procedure followed that of porous silicon samples used in other studies.[9–11] One of these studies provided a value of $\kappa = (1.87 \pm 0.08) \times 10^{-17}\,\mathrm{m^2\,Pa^{-1}\,s^{-1}}$, measured by studying the lateral, steady-state, negative-pressure-driven flow of water through sealed layers of porous silicon with a microfluidic approach.[10] We assume that the permeability in our case should be similar, in particular because the capillary pressure, equilibrium contact angle and porosity measured in the aforementioned study ($\Delta P_\mathrm{c} = (-76 \pm 5)$ MPa, $\theta_\mathrm{e} = (25 \pm 5)°$, $\phi = 0.45$, respectively) are very close to the values we have obtained on our material, and the working temperature was also comparable, $(22.5 \pm 2.5)\,°\mathrm{C}$. Eventually, from Equation S20, we obtain

$$w = (7.0 \pm 1.1) \times 10^{-9}\,\mathrm{m^2/s} \tag{S21}$$

as the estimated LW coefficient for our material. This value is comparable to experimental values for $w$ obtained in other studies.[10,11]

## S3.3 Droplet: initial transient

The initial transient seen in droplet volumetric data may be due to several effects.

**Vertical imbibition** First, the porous medium below the droplet initially absorbs a volume, $\Delta V_0 = \pi R_\mathrm{drop}^2 H \phi = 0.011\,\mathrm{\mu L}$ due to vertical capillary imbibition from the droplet into the pores, i.e., $\Delta V_0/V_0 \simeq 1\,\%$. Also, the timescale of that process is $H^2/w \simeq 3\,\mathrm{ms}$ from the LW Equation, using a typical value $w = 7 \times 10^{-9}\,\mathrm{m^2/s}$ based on material properties (see *Lucas-Washburn coefficient above*). As a result, this step of vertical imbibition should

not be visible in our experiments both in terms of impacted volumes and time resolution.

**Halo development** The initial transient is thus most likely due to halo formation, since part of the droplet's liquid is sucked into the pores by imbibition. Indeed, the timescales of this transient are similar to the values of $\tau$ for halo formation (see Main Text). Also, the volume of liquid sucked in the porous medium (below the droplet and in the halo) is on the order of $\Delta V = \pi \left[ (R_{\text{drop}} + L_{\text{max}})^2 - R_{\text{drop}}^2 \right] H\phi$ with $R = R_{\text{drop}} + L_{\text{max}}$. We estimate $\Delta V / V_0 \simeq$ 1-– 10% using the halo extension data of Figure 7c (Main Text), which is comparable to the initial volume drops seen in the Main Text (Figure 8a).

# S4 Misc. discussion

## S4.1 Fitting of halo dynamics

As described in the Main Text, we added an initial time shift, $t_0$ as a free parameter in the fitting procedure for best results, i.e. we fitted the $L_{\text{eff}}^2(t)$ data with

$$L_{\text{eff}}^2(t) = w\tau \left( 1 - \exp\left( -\frac{t - t_0}{\tau} \right) \right) \quad \text{(S22)}$$

The resulting time shifts were small, with $t_0 = 1\,\text{s}$ at 5%RH up to $t_0 = 4\,\text{s}$ at 50%RH and $t_0 = 10\,\text{s}$ at 60%RH, or $t_0/\tau \simeq 0.1$ for all RH. The necessity of this procedure came from the fact that the dynamics of the halo at very short times was closer to being linear for $L(t)$ rather than linear for $L^2(t)$, as can be seen in Figure 6a (Main Text). This observation suggests that an additional physical mechanisms might limit the dynamics at very short times, or points to halo detection problems when the imbibition front is too close to the droplet. Nevertheless, since $t0 \ll \tau$, we do not expect significant impact of this time shift on the interpretation of our results. The rescaled data (Figure 6c, Main Text), where $t_0$ is not subtracted, also shows that these initial deviations only resulted in small departures to the dynamics predicted by the model.

## S4.2 Dynamic vs. equilibrium humidity

The fact that $\mathcal{H}_{\text{eq}}$ extracted from halo timescales lies in the upper range of values estimated from isotherms might originate from two effects, potentially combined. First, since we define the halo as being at the edge of the fully wet zone on the experimental images (see *Methods* in Main Text), this corresponds thermodynamically to a point of the isotherm at the evaporation point but still at filling fraction of 1, i.e. at the right side of the evaporation range in the isotherm (Main Text, Figure 2, shaded blue area). Second, as mentioned in the Main Text (see *Theory*), the curvature of the menisci in the pores should not be identical across the halo, due to liquid pressure gradients in the pores. According to the Kelvin equation, these variations would cause differences in equilibrium RH depending on the position of the halo, with higher equilibrium RH closer to the droplet. Such an effect may cause an average equilibrium RH in the halo larger than that estimated from isotherms, for which there is no gradients in pressure or curvature.

# References


(1) Bellezza, H.; Poizat, M.; Vincent, O. Salt Crystallization and Deliquescence Triggered by Humidity Cycles in Nanopores. *submitted* **2025**,

(2) Bossert, M.; Grosman, A.; Trimaille, I.; Noûs, C.; Rolley, E. Stress or Strain Does Not Impact Sorption in Stiff Mesoporous Materials. *Langmuir* **2020**, *36*, 11054–11060.

(3) Bellezza, H. Changements de Phase de Solutions Salées Induits Par Des Cycles d'humidité En Milieux Nanoporeux : Évaporation, Condensation, Cristallisation et Déliquescence. Ph.D. thesis, Université Claude Bernard Lyon 1, Institut Lumière Matière, 2023.

(4) Thommes, M.; Cychosz, K. A. Physical Adsorption Characterization of Nanoporous Materials: Progress and Challenges. *Adsorption* **2014**, *20*, 233–250.

(5) Schwarz, D.; Wormeester, H.; Poelsema, B. Validity of Lorentz–Lorenz Equation in Porosimetry Studies. *Thin Solid Films* **2011**, *519*, 2994–2997.

(6) Markel, V. A. Introduction to the Maxwell Garnett Approximation: Tutorial. *Journal of the Optical Society of America A* **2016**, *33*, 1244.

(7) Polyanskiy, M. N. Refractiveindex.Info Database of Optical Constants. *Scientific Data* **2024**, *11*, 94.

(8) Kitamura, N.; Fukumi, K.; Nishii, J.; Ohno, N. Relationship between Refractive Index and Density of Synthetic Silica Glasses. *Journal of Applied Physics* **2007**, *101*, 123533.

(9) Vincent, O.; Sessoms, D. A.; Huber, E. J.; Guioth, J.; Stroock, A. D. Drying by Cavitation and Poroelastic Relaxations in Porous Media with Macroscopic Pores Connected by Nanoscale Throats. *Physical Review Letters* **2014**, *113*, 134501.

(10) Vincent, O.; Szenicer, A.; Stroock, A. D. Capillarity-Driven Flows at the Continuum Limit. *Soft Matter* **2016**, *12*, 6656–6661.

(11) Vincent, O.; Marguet, B.; Stroock, A. D. Imbibition Triggered by Capillary Condensation in Nanopores. *Langmuir* **2017**, *33*, 1655–1661.

(12) Steiger, M.; Kiekbusch, J.; Nicolai, A. An Improved Model Incorporating Pitzer's Equations for Calculation of Thermodynamic Properties of Pore Solutions Implemented into an Efficient Program Code. *Construction and Building Materials* **2008**, *22*, 1841–1850.

(13) Krumgalz, B. S.; Pogorelsky, R.; Pitzer, K. S. Volumetric Properties of Single Aqueous Electrolytes from Zero to Saturation Concentration at 298.15 °K Represented by Pitzer's Ion-Interaction Equations. *Journal of Physical and Chemical Reference Data* **1996**, *25*, 663–689.

(14) Pátek, J.; Hrubý, J.; Klomfar, J.; Součková, M.; Harvey, A. H. Reference Correlations for Thermophysical Properties of Liquid Water at 0.1MPa. *Journal of Physical and Chemical Reference Data* **2009**, *38*, 21–29.

(15) Wagner, W.; Pruß, A. The IAPWS Formulation 1995 for the Thermodynamic Properties of Ordinary Water Substance for General and Scientific Use. *Journal of Physical and Chemical Reference Data* **2002**, *31*, 387–535.

(16) Petrova, T.; Dooley, RB. Revised Release on Surface Tension of Ordinary Water Substance. *Proceedings of the International Association for the Properties of Water and Steam, Moscow, Russia* **2014**, *63*, 23–27.

(17) Massman, W. J. A Review of the Molecular Diffusivities of H2O, CO2, CH4, CO, O3, SO2, NH3, N2O, NO, and NO2 in Air, O2 and N2 near STP. *Atmospheric Environment* **1998**, *32*, 1111–1127.

(18) Vincent, O. Python Aquasol v.1.7.1. https://pypi.org/project/aquasol, 2025.
